# Supplementary material for: The HI and stellar mass bivariate distribution of centrals and satellites for all, late- and early-type local galaxies
Source: arXiv:2104.01983 source file (2021-05-26)
Supplement: Supplementary file 1 [file supplementary_material.pdf]

# Supplementary material

This supplementary material corresponds to the paper entitled "The HI and stellar mass bivariate distribution of centrals and satellites for all, late- and early-type local galaxies" by Calette et al. (2021).

## S.M.1 Conditional Probability Distributions Functions

Figures S1-S3 show the $R_{\rm HI}$ ($\equiv$ $M_{\rm HI}/M_*$) probability density distribution functions (PDFs) at different stellar masses (indicated in parenthesis in each panel) for all, late-type, and early-type galaxies from our empirically-constrained model (as described in Section 3.3 of the manuscript). In every figure the solid, dashed and dotted lines correspond to all, central and satellite galaxies, respectively. The first two panels are in gray to indicate that for these masses the distributions of centrals and satellites are extrapolations from our constrains using the `xGASS` survey. For comparison, we include the `xGASS` PDFs after applying the corrections and survival analysis discussed in §§2.2–2.4 of the manuscript. These correspond to the CDFs presented in Figures 5-7 within the given stellar mass bins as indicated. In the panels in which upper limits dominate over detections, the `xGASS` PDFs are shown with the left-side open histograms. The error bars in the histograms show the Poissonian error from the count. Note that the `xGASS` PDFs are measured within mass intervals of $\approx$ 0.31 dex wide, while our empirical determinations are shown for the central mass from each interval.

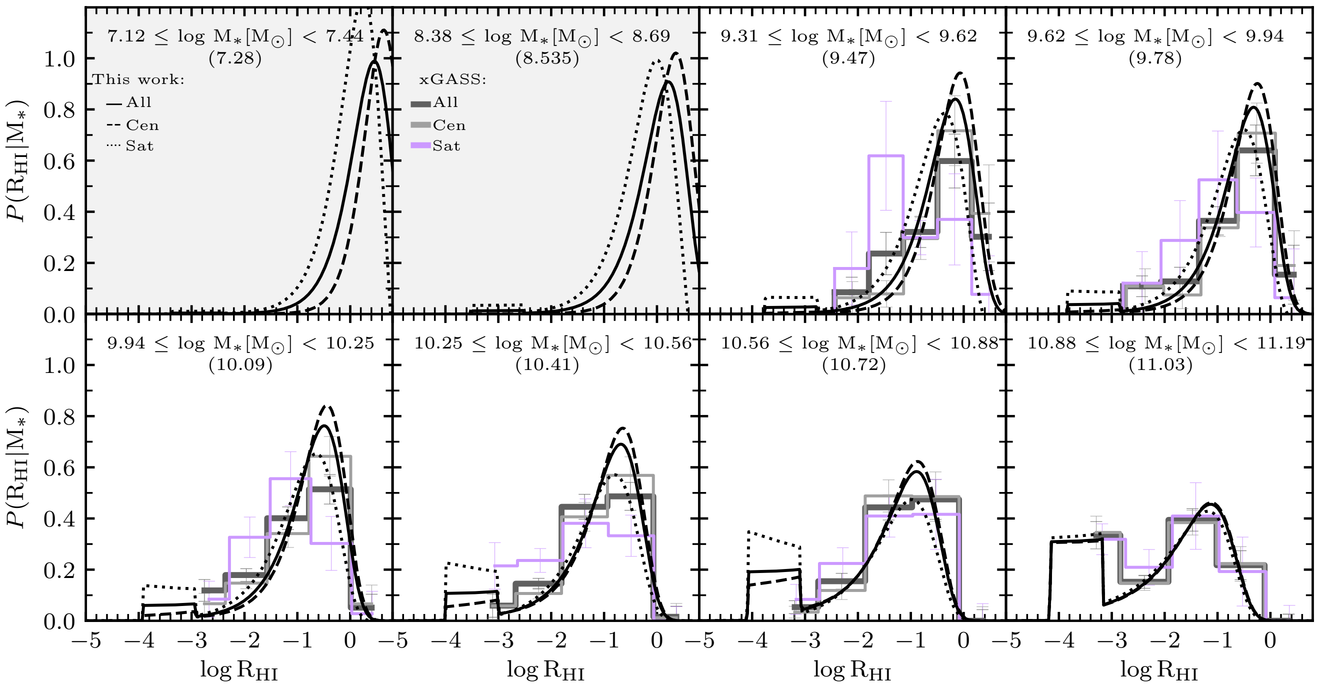


**Figure S1:** $R_{\rm HI}$ PDFs of all galaxies as a function of stellar mass; the $\log(M_*/{\rm M}_\odot)$ is shown in parenthesis at each panel. Black solid, dashed and dotted lines correspond to our empirically-constrained $R_{\rm HI}$ PDFs for all, central, and satellite galaxies, respectively. We also show the `xGASS` PDFs within the stellar mass bins indicated in each panel. These PDFs correspond to the $R_{\rm HI}$ cumulative distributions presented in Figure 5 from the main manuscript. The first two panels show our PDFs extrapolated to lower stellar masses.

The xGASS $R_{\rm HI}$ distributions are only marginally described by our empirical model. Recall that this model was constrained with a large set of observational samples, including xGASS. However, our empirically-constrained PDFs capture the systematic differences from the xGASS survey, within the uncertainties, between centrals and satellites as a function of stellar mass, which was the goal of our exercise using the xGASS survey.

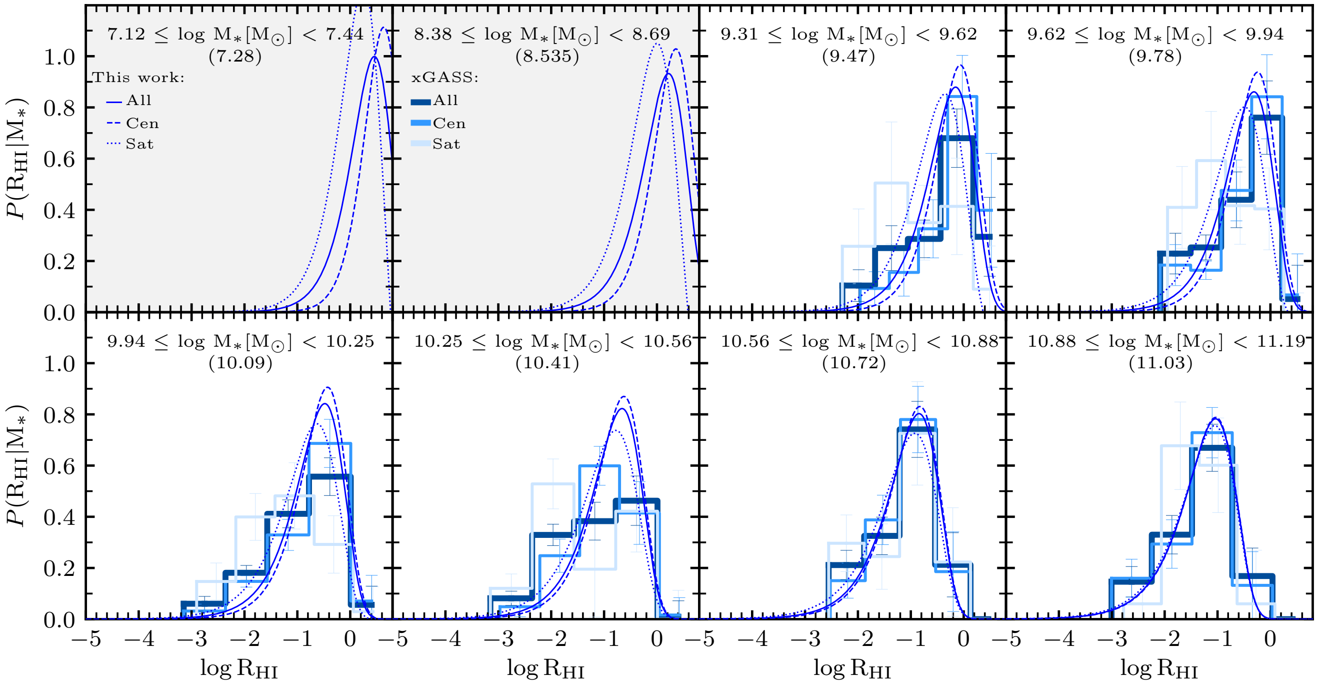


**Figure S2:** Same as Figure S1 but for LTGs.

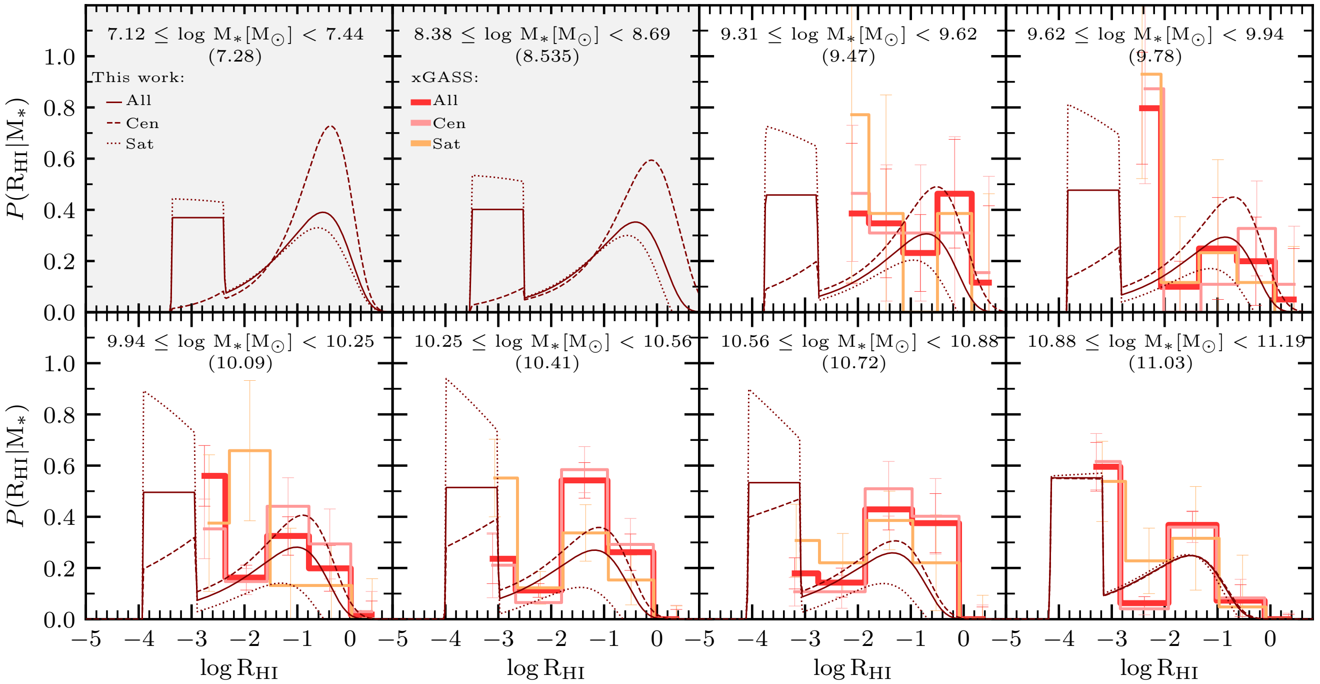


**Figure S3:** Same as Figure S1 but for ETGs.

### S.M.2 Additional data tables

Below we tabulate the electronic data corresponding to selected figures from the manuscript.

Table S1 provides the data of the xGASS fractions plotted in panels (c) and (d) of Figure 2: $f_c^L$, the fraction of late-type galaxies that are centrals; $f_s^L$, the fraction of late-type galaxies that are satellites; $f_c^E$, the fraction of early-type galaxies that are centrals; and, $f_s^E$, the fraction of early-type galaxies that are satellites,

Table S2 provide the data corresponding to the $\langle \log \mathrm{R_{HI}} \rangle$-log $M_*$ correlation for all galaxies from the xGASS survey. Columns (2) and (3) are the values when including upper-limits, volume and environment corrections (panel c of Figure 3). Columns (4) and (5) do not include any correction (panel c of Figure C1). Columns (6) and (7) include corrections to upper limits only (panel i of Figure C1).

Table S3 is as Table S2 but for late-type galaxies and corresponds to panel (a) of Figures 3 and panels (a) and (g) of Figure C1.

Table S4 is as Table S2 but for early-type galaxies and corresponds to panel (b) of Figures 3 and panels (b) and (h) of Figure C1. Note that when we do include any correction to the xGASS data the means above $M_* \sim 5 \times 10^9$ $\mathrm{M_\odot}$ are only an estimate of the upper bound, therefore, error on the means (or Error of the deviations) are meaningless (see Appendix C of the manuscript).

**Table S1:** xGASS fractions as presented in panels (c) and (d) of Figure 2.

| $\log M_*$ (1) | $f_c^L$ (2) | $f_s^L$ (3) | $f_c^E$ (4) | $f_s^E$ (5) |
|---|---|---|---|---|
| 9.16 | 0.73 | 0.26 | 0.51 | 0.49 |
| 9.47 | 0.70 | 0.30 | 0.51 | 0.50 |
| 9.78 | 0.78 | 0.22 | 0.59 | 0.41 |
| 10.09 | 0.70 | 0.30 | 0.58 | 0.42 |
| 10.41 | 0.71 | 0.29 | 0.57 | 0.43 |
| 10.72 | 0.71 | 0.29 | 0.61 | 0.39 |
| 11.03 | 0.67 | 0.33 | 0.77 | 0.23 |
| 11.34 | 0.79 | 0.21 | 0.95 | 0.05 |

**Table S2:** `xGASS` $\langle \log \mathrm{R_{HI}} \rangle$-$\log M_*$ relations for all galaxies.

| $\log M_*$ | $\langle \log \mathrm{R_{HI}} \rangle$ | Error of the mean (SD) | $\langle \log \mathrm{R_{HI}} \rangle$ | Error of the mean (SD) | $\langle \log \mathrm{R_{HI}} \rangle$ | Error of the mean (SD) |
|---|---|---|---|---|---|---|
| | corrs: u.l.+Vol+env | | no corr | | corrs: u.l. | |
| (1) | (2) | (3) | (4) | (5) | (6) | (7) |
| 9.16 | -0.27 | 0.004 (0.67) | -0.26 | 0.055 (0.65) | -0.30 | 0.062 (0.73) |
| 9.47 | -0.50 | 0.004 (0.72) | -0.58 | 0.076 (0.84) | -0.65 | 0.088 (0.97) |
| 9.78 | -0.67 | 0.004 (0.79) | -0.73 | 0.067 (0.76) | -0.90 | 0.094 (1.06) |
| 10.10 | -1.06 | 0.003 (0.74) | -1.08 | 0.046 (0.74) | -1.26 | 0.066 (1.05) |
| 10.41 | -1.40 | 0.005 (1.04) | -1.28 | 0.041 (0.63) | -1.63 | 0.076 (1.16) |
| 10.72 | -1.59 | 0.007 (1.10) | -1.32 | 0.040 (0.59) | -1.73 | 0.082 (1.21) |
| 11.04 | -2.54 | 0.015 (1.08) | -1.65 | 0.052 (0.77) | -2.10 | 0.083 (1.23) |

**Table S3:** `xGASS` $\langle \log \mathrm{R_{HI}} \rangle$-$\log M_*$ relations for late-type galaxies.

| $\log M_*$ | $\langle \log \mathrm{R_{HI}} \rangle$ | Error of the mean (SD) | $\langle \log \mathrm{R_{HI}} \rangle$ | Error of the mean (SD) | $\langle \log \mathrm{R_{HI}} \rangle$ | Error of the mean (SD) |
|---|---|---|---|---|---|---|
| | corrs: u.l.+Vol+env | | no corr | | corrs: u.l. | |
| (1) | (2) | (3) | (4) | (5) | (6) | (7) |
| 9.16 | -0.25 | 0.004 (0.66) | -0.21 | 0.055 (0.61) | -0.24 | 0.061 (0.68) |
| 9.47 | -0.44 | 0.004 (0.70) | -0.46 | 0.080 (0.80) | -0.46 | 0.081 (0.81) |
| 9.78 | -0.57 | 0.003 (0.57) | -0.51 | 0.064 (0.63) | -0.53 | 0.069 (0.68) |
| 10.10 | -0.94 | 0.003 (0.69) | -0.91 | 0.053 (0.71) | -0.94 | 0.059 (0.79) |
| 10.41 | -1.18 | 0.004 (0.74) | -1.06 | 0.053 (0.62) | -1.14 | 0.067 (0.78) |
| 10.72 | -1.13 | 0.005 (0.61) | -1.07 | 0.050 (0.53) | -1.11 | 0.058 (0.61) |
| 11.04 | -1.42 | 0.007 (0.69) | -1.37 | 0.064 (0.66) | -1.42 | 0.071 (0.73) |

**Table S4:** `xGASS` $\langle \log \mathrm{R_{HI}} \rangle$-$\log M_*$ relations for early-type galaxies.

| $\log M_*$ | $\langle \log \mathrm{R_{HI}} \rangle$ | Error of the mean (SD) | $\langle \log \mathrm{R_{HI}} \rangle$ | Error of the mean (SD) | $\langle \log \mathrm{R_{HI}} \rangle$ | Error of the mean (SD) |
|---|---|---|---|---|---|---|
| | corrs: u.l.+Vol+env | | no corr | | corrs: u.l. | |
| (1) | (2) | (3) | (4) | (5) | (6) | (7) |
| 9.16 | -0.79 | 0.024 (0.86) | -0.67 | 0.185 (0.90) | -0.79 | 0.235 (1.14) |
| 9.47 | -1.42 | 0.023 (1.05) | -1.10 | 0.166 (0.96) | -1.42 | 0.229 (1.32) |
| 9.78 | -1.91 | 0.019 (1.03) | -1.34 | - | -1.91 | 0.193 (1.26) |
| 10.10 | -1.97 | 0.013 (1.10) | -1.44 | - | -1.97 | 0.128 (1.22) |
| 10.41 | -2.23 | 0.012 (1.14) | -1.53 | - | -2.23 | 0.122 (1.29) |
| 10.72 | -2.29 | 0.012 (1.19) | -1.56 | - | -2.29 | 0.122 (1.34) |
| 11.04 | -2.65 | 0.011 (1.18) | -1.85 | - | -2.65 | 0.112 (1.27) |
